# Supplementary material for: Valley Plasmonics in the Dichalcogenides
Source: arXiv:1601.01707 source file (2016-01-07)
Supplement: Supplementary file 1 [file Supplement.pdf]

# Supplemental Material to: Valley Plasmonics in the Dichalcogenides

R. E. Groenewald,[1] M. Rösner,[2,3] G. Schönhoff,[2,3] S. Haas,[1] and T. O. Wehling[2,3]

[1]*Department of Physics and Astronomy, University of Southern California, Los Angeles, CA 90089-0484, USA*
[2]*Institut für Theoretische Physik, Universität Bremen, Otto-Hahn-Allee 1, 28359 Bremen, Germany*
[3]*Bremen Center for Computational Materials Science, Universität Bremen, Am Fallturm 1a, 28359 Bremen, Germany*

(Dated: January 7, 2016)

## BAND STRUCTURE OF THE EFFECTIVE THREE BAND MODEL

In Fig. 1 we show the band structure in the basis of the three predominant Mo $d$ orbitals for $MoS_2$ with and without spin orbit coupling (SOC). The SOC is included as describe in [1] with $\lambda = 0.1\,\mathrm{eV}$ as the SOC coefficient. All of these three bands are actually entangled and hybridized with the missing molybdenum $d$ orbitals as well as sulfur $p$ orbitals. To get well defined electronic bands, we use the Wannier90 package [2] in order to properly disentangle the bands. Thereby we use a "frozen" or "inner" energy window, which fixes the $G_0W_0$ valence-band's energy as well as most parts of the lowest conduction band. Afterwards we stay with the resulting projections without performing a maximal localization.

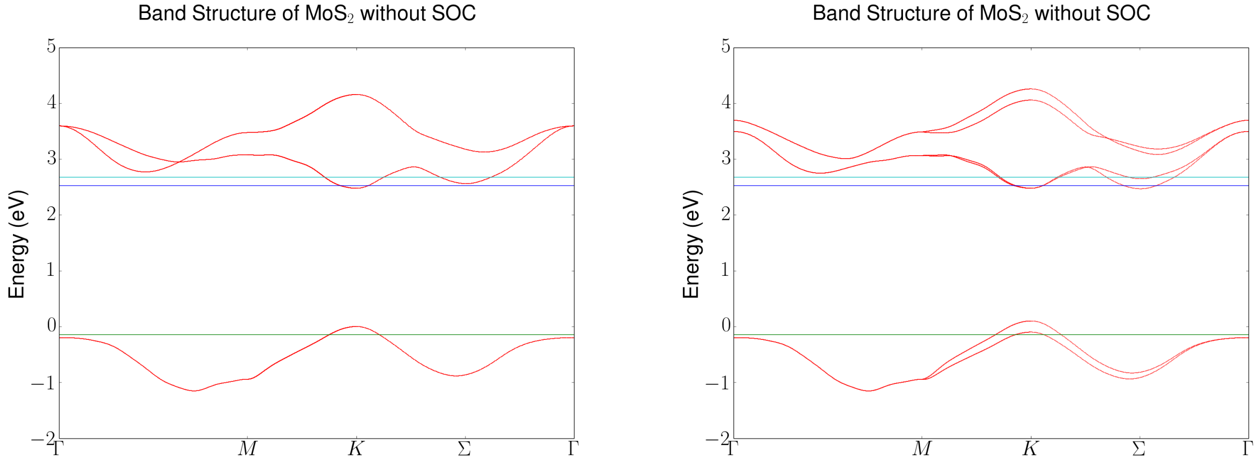


Figure 1: (Color online) Band structure of $MoS_2$ without (left) and with (right) spin orbit coupling. The two lowest conduction bands and highest valence band are shown. Note the direct band gap at $K$ and valleys at $\Sigma$. The doping levels discussed in the main text are shown with horizontal lines: green (hole doping) $E_f = -0.15\,\mathrm{eV}$, blue (low electron doping) $E_f = 2.52\,\mathrm{eV}$ and cyan (high electron doping) $E_f = 2.67\,\mathrm{eV}$. With SOC the spin degeneracy at $K$ and $K'$ in the valence band and at $\Sigma$ and $\Sigma'$ in the lowest conduction band is lifted. These splittings are responsible for gapped inter-valley plasmon dispersions as discussed in the main text.

The doping levels were selected such that in the hole doped case both $K$ and $K'$ are occupied when SOC is included and similarly for the high electron doped case ($E_f = 2.67eV$) such that both $\Sigma$ and $\Sigma'$ will be occupied. Since only $d_{xy}$ and $d_{x^2-y^2}$ orbitals are affected by spin orbit coupling, only those parts of the band structure splits upon SOC inclusion which have a non-vanishing $d_{xy}$ or $d_{x^2-y^2}$ character.

## BENCHMARKS

Up to now, there have been basically two theoretical approaches available to study the plasmonic physics in TMDCs. On the one side there are models combining effective $k \cdot p$ descriptions of the quadratic electronic bands around the band gap with an evaluation of the dielectric function within the random phase approximation (RPA) [3, 4]. On the other side, there are RPA descriptions based on full density functional theory (DFT) calculations, which include realistic single particle band structures describing the complete Brillouin zone [5–10].

Here, we add a third approach by utilizing a material-specific low-energy model Hamiltonian derived from ab initio calculations for the undoped material as the basis for the evaluation of dynamical response functions in the electron and hole doped situations. Thereby we gain the possibility to accurately calculate the polarization as well as the screening functions for the whole Brillouin zone, which enables us to study plasmons at arbitrary momenta as described in the main text.

In Fig. 2 we compare the resulting plasmon dispersions of our ab initio based model (dots) to the models by Scholz et al. [3] and Kechedzhi et al. [4] (lines) for hole doping with a carrier density of $2 \times 10^{13}\mathrm{cm}^{-2}$ in the case of $MoS_2$. In the $k \cdot p$ models a simple *constantly screened* Coulomb interaction of the form $U(q) \propto \frac{1}{\kappa q}$ with $\varepsilon_{\alpha\beta}(\mathbf{q}) = \kappa = 5$ is used. As long as we use the same constantly screened Coulomb interaction to evaluate the dielectric function we end up with nearly identical plasmon dispersions compared to those derived from the $k \cdot p$-models. However, by including the full ab initio derived $q$ dependent dielectric function for the background screening in the undoped case, which arises due to the two dimensional geometry and the *excluded* bands, we find strongly reduced plasmon energies (green dots).

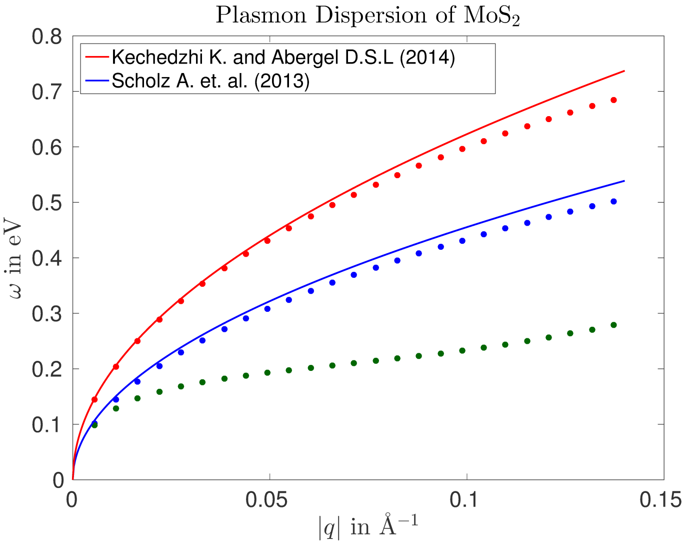


Figure 2: (Color online) Plasmon dispersions from our ab initio based model (dots) in comparison with analytics $k \cdot p$-models by Scholz et al. [3] and Kechedzhi et al. [4]. In both $k \cdot p$-models the authors used a simple $\frac{1}{\kappa q}$ constantly screened Coulomb potential while we take the full background screened Coulomb interaction into account (green dots). When we switch to the same constantly screened Coulomb potential our results match those of the other authors as seen by the red and blue dots respectively. The two $k \cdot p$-models produce different plasmon dispersions due to the ways they handle the spin dependencies. In the data by Kechedzhi et al. [4] both spin components and their coupling are included while the data of Scholz et al. [3] include a single spin component only.

In Fig. 3 we compare our method to full ab initio results for $NbS_2$ [8], which is a metal in its ground state. Once again, plasmon dispersions derived form EELS data are shown. Although, the resulting plasmon dispersion are on the eV range (for which our model is actually not set-up), we find a remarkable agreement with differences on the order of 100 meV to 200 meV ($\approx 10\%$ to $20\%$). Hence, we conclude that neglecting the material-specific dielectric function $\varepsilon_{\alpha\beta}(\mathbf{q})$ within the minimal three-band model is a crucial approximation leading to non-realistic plasmonic properties.

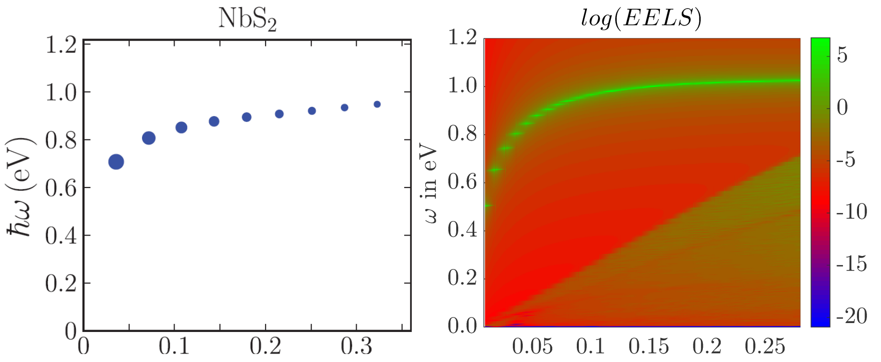


Figure 3: (Color online) Plasmon dispersions for undoped $NbS_2$ from (left) full ab initio calculations from [8] and (right) our ab initio based model. Here we use the macroscopic dielectric function.

## ELECTRON DOPED WITHOUT SOC

The polarization for $d_{z^2} - d_{z^2}$ scattering is shown in Fig. 4 for high electron doping (such that $K$ and $\Sigma$ valleys are partially occupied). The doping here corresponds to that in Fig. 3 (b) of the main text. We point out the resonances around $\mathbf{q} = \mathbf{K}$ are due to scattering from one $K$ valley to another (unlike the resonances at $K$ in the main text which corresponds to scattering between $\Sigma$ valleys). Also, the nascent excitations at $\Sigma$ and $M$ are much stronger in this case [as compared to the low electron doping case in the main text shown in Fig. 3 (a)] because the doping is so high that the $\Sigma$ valleys carry significantly more $d_{z^2}$ character. These excitations are no longer gapped because the doping is high enough that $\Sigma$ valleys are also occupied.

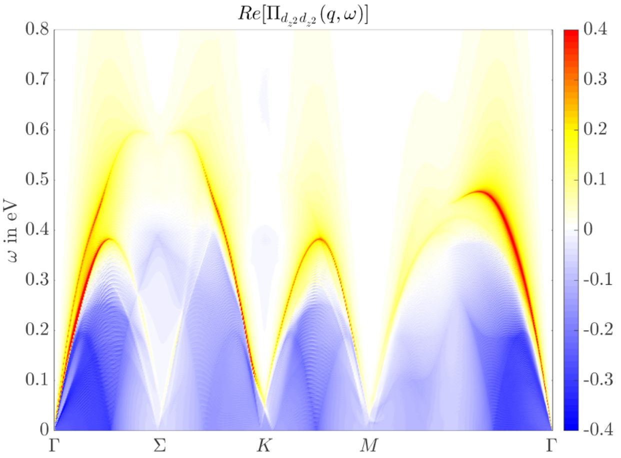


Figure 4: (Color online) Polarization for electron doping with $E_f = 2.67\,\text{eV}$ due to $d_{z^2} - d_{z^2}$ scattering. The *inter-valley* transitions from $K$ to $K'$ is seen by the resonances around $\mathbf{q} = \mathbf{K}$. Note that we also find an excitation at $\mathbf{q} = \mathbf{M}$ (and a weak one at $\mathbf{q} = \mathbf{\Sigma}$), this is due to the fact that at $E_f = 2.67\,\text{eV}$ the system is so heavily doped that we enter a region where the $\Sigma$ valleys also carry considerable $d_{z^2}$ character and therefore we see $\Sigma - \Sigma'$ *inter-valley* transitions even in $\Pi_{d_{z^2}d_{z^2}}$.


[1] G.-B. Liu, W.-Y. Shan, Y. Yao, W. Yao, and D. Xiao, Physical Review B **88**, 085433 (2013).
[2] A. A. Mostofi, J. R. Yates, Y.-S. Lee, I. Souza, D. Vanderbilt, and N. Marzari, Computer Physics Communications **178**, 685 (2008).
[3] A. Scholz, T. Stauber, and J. Schliemann, Physical Review B **88**, 035135 (2013).
[4] K. Kechedzhi and D. S. L. Abergel, Physical Review B **89**, 235420 (2014).
[5] P. Johari and V. B. Shenoy, ACS Nano **5**, 5903 (2011).
[6] M. N. Faraggi, A. Arnau, and V. M. Silkin, Physical Review B **86**, 035115 (2012).
[7] P. Cudazzo, M. Gatti, and A. Rubio, Physical Review B **86**, 075121 (2012).

[8] K. Andersen and K. S. Thygesen, Physical Review B **88**, 155128 (2013).
[9] P. Cudazzo, M. Gatti, and A. Rubio, Physical Review B **90**, 205128 (2014).
[10] Y. Liang and L. Yang, Physical Review Letters **114**, 063001 (2015).
